# Supplementary material for: Nanopteron-stegoton traveling waves in spring dimer Fermi-Pasta-Ulam-Tsingou lattices
Source: arXiv:1710.07376 source file (2017-10-20)
Supplement: Supplementary file 1 [file appendix_operator_conjugation.tex]

%%------------------------------------------------------------------------------------------------------------------------------------------------------------------------------------------------------------%%
%%------------------------------------------------------------------------------------------------------------------------------------------------------------------------------------------------------------%%
%%------------------------------------------------------------------------------------------------------------------------------------------------------------------------------------------------------------%%
\subsubsection{Operator conjugation} Our goal in this section is to extend a Fourier multiplier defined on $H^r$ to map (a subspace of) $H_q^r$ into $H_q^r$. 
%For brevity, let $c_q(x) = \cosh(qx)$ and $s_q(x) = \sech(qx)$.  
With these preliminaries underway, we can now state our major tool, which is a lemma by Beale \cite{beale1} (Lemma 3), \cite{beale2} (Lemma 5.1).

%%------------------------------------------------------------------------------------------------------------------------------------------------------------------------------------------------------------%%
%%------------------------------------------------------------------------------------------------------------------------------------------------------------------------------------------------------------%%
\begin{theorem}[Beale]
Let $q > 0$ and let $\tmu$ be meromorphic on the strip
$$
\overline{\Sigma}_q = \set{z \in \C}{|\im(z)| \le q}
$$
with the following properties.

%%------------------------------------------------------------------------------------------------------------------------------------------------------------------------------------------------------------%%
%%------------------------------------------------------------------------------------------------------------------------------------------------------------------------------------------------------------%%
\begin{enumerate}[label={\bf(\roman*)}]
%%------------------------------------------------------------------------------------------------------------------------------------------------------------------------------------------------------------%%
\item Let $P_{\mu}$ be the set of poles of $\tmu$ in $\overline{\Sigma}_q$.  Suppose that $\tmu$ has a finite number of poles in $\overline{\Sigma}_q$, all of which are real and simple.   
%%------------------------------------------------------------------------------------------------------------------------------------------------------------------------------------------------------------%%
\item Let $s \ge 0$ and $C,$ $z_0 > 0$ such that if $|z| \ge z_0$, then
$$
|\tmu(z)| \le \frac{C}{|\re(z)|^s}.
$$
\end{enumerate}
Let $r \ge 0$ and set
$$
\mathfrak{D}_{\mu,q}^{r} := \set{f \in H_q^r}{z \in P_{\mu} \Longrightarrow \hat{f}(z) = 0}
$$
and let $\mu$ be the Fourier multiplier with symbol $\tmu$.  Then $\mu \in \b(\mathfrak{D}_{\mu,q}^r,H_q^{r+s})$ and
$$
\norm{\mu{f}}_{r+s,q} \le \left(\sup_{\substack{z \in \mathbb{C} \\ |\im(z)| = q}} (1+|\re(z)|^2)^{s/2}|\tmu(z)|\right)\norm{f}_{r,q}.
$$
\end{theorem}

We apply Beale's lemma to prove the following. 

%In a similarly weighted problem, P\&W observe equivalence by conjugating the operators with exponential weights cf. eq 1.15 \cite{pego-weinstein}

%%------------------------------------------------------------------------------------------------------------------------------------------------------------------------------------------------------------%%
%%------------------------------------------------------------------------------------------------------------------------------------------------------------------------------------------------------------%%
\begin{proposition}[Operator conjugation]\label{operator conjugation}
Suppose that $\tmu$ satisfies the hypotheses of Beale's lemma on the closed strip $\overline{\Sigma}_q$ and that there are constants $q_0$, $C > 0$ such that
$$
|\tmu(k+ iq) - \tmu(k)| \le C|q|
$$
for all $q \in (-q_0,q_0)$.  Let $\mu$ be the Fourier multiplier with symbol $\tmu$ and set $c_q(x) = \cosh(qx)$ and $s_q(x) = \sech(qx)$. Then $\mu_q := c_q\mu[s_q\cdot] \in \b(H^r,H^r)$ and 
\begin{equation}\label{operator conj limit}
\lim_{q \to 0^+} \norm{\mu_q-\mu}_{\b(H^r,H^r)} = 0.
\end{equation}
\end{proposition}

\begin{proof}
First we show that $\mu_q$ is a well-defined operator on $H^r$.  Fix $f \in H^r$, so $s_qf \in H_q^r$.  Beale's lemma tells us that $\mu$ maps $H_q^r$ to $H_q^r$ for $q$ in some interval $(0,q_{\mathsf{B}})$, so $\mu[s_qf] \in H_q^r$, and consequently $\mu_qf = c_q\mu[s_qf] \in H^r$, too.

For the limit, we compute
$$
\norm{c_q\mu[s_qf]-\mu[f]}_{H^r}^2
= \int_{\R} (1+k^2)^r|\ft[c_q\mu[s_qf]-\mu[f]](k)|^2 \dk.
$$
By \eqref{complex ft defn at q}, we have
$$
\ft[c_q\mu[s_qf]](k)
= \frac{\ft[\mu[s_qf]](k+iq) + \ft[\mu[s_qf]](k-iq)}{2},
$$
and since $\mu$ is a Fourier multiplier, this becomes
$$
\ft[c_q\mu[s_qf]](k)
= \frac{\tmu(k+iq)\hat{s_qf}(k+iq) + \tmu(k-iq)\hat{s_qf}(k-iq)}{2}.
$$

Next, since $c_qs_q = 1$, we have
$$
\hat{f}(k)
= \hat{c_qs_qf}(k)
= \frac{\hat{s_qf}(k+iq) + \hat{s_qf}(k-iq)}{2},
$$
and so
$$
\hat{\mu{f}}(k) 
= \tmu(k)\hat{f}(k)
= \tmu(k)\frac{\hat{s_qf}(k+iq) + \hat{s_qf}(k-iq)}{2}.
$$
Then
\begin{align*}
\ft[c_q\mu[s_qf]-\mu[f]](k)
&= \frac{\tmu(k+iq)\hat{s_qf}(k+iq) + \tmu(k-iq)\hat{s_qf}(k-iq)}{2}
-\tmu(k)\frac{\hat{s_qf}(k+iq) + \hat{s_qf}(k-iq)}{2} \\
\\
&= \left(\tmu(k+iq)-\tmu(k)\right)\frac{\hat{s_qf}(k+iq)}{2}
+ \left(\tmu(k-iq)-\tmu(k)\right)\frac{\hat{s_qf}(k-iq)}{2}.
\end{align*}
By hypothesis on $\tmu$, we have
$$
\left|\left(\tmu(k\pm iq)-\tmu(k)\right)\frac{\hat{s_qf}(k\pm iq)}{2}\right|
\le Cq\left|\hat{s_qf}(k \pm iq)\right|
= Cq|\ft[e^{\pm{q}\cdot}s_qf](k)|.
$$

Now define the multiplication operator
$$
T_q \colon H^r \to H^r \colon f \mapsto e^{q\cdot}s_qf.
$$
This is not a Fourier multiplier but just an ordinary multiplication operator, and so
$$
\norm{T_q}_{\b(H^r,H^r)} \le C_r\norm{e^{q\cdot}s_q}_{W^{r,\infty}}.
$$
Using the bound on this $W^{r,\infty}$-norm from Lemma \ref{eq sq fdb} below, we conclude
\begin{align*}
\norm{c_q\mu[s_qf]-\mu[f]}_{H^r}^2
&= \int_{\R} (1+k^2)^r|\ft[c_q\mu[s_qf]-\mu[f]](k)|^2 \dk \\
\\
&= \int_{\R}(1+k^2)^r\left| \left(\tmu(k+iq)-\tmu(k)\right)\frac{\hat{s_qf}(k+iq)}{2}\right|^2 \dk \\
\\
&+ \int_{\R}(1+k^2)^r\left|\left(\tmu(k-iq)-\tmu(k)\right)\frac{\hat{s_qf}(k-iq)}{2}\right|^2 \dk \\
\\
&\le Cq\int_{\R}(1+k^2)^r|\hat{T_qf}(k)|^2 \dk + Cq\int_{\R}(1+k^2)^r|\hat{T_{-q}f}(k)|^2 \dk \\
\\
&= Cq\norm{T_qf}_{H^r}^2 + Cq\norm{T_{-q}f}_{H^r}^2 \\
\\
&\le Cq\norm{T_q}_{\b(H^r,H^r)}^2 + Cq\norm{T_{-q}}_{\b(H^r,H^r)}^2 \text{ since } \norm{f}_{H^r} \le 1 \\
\\
&\le C_rq. 
\end{align*}
This inequality proves the limit \eqref{operator conj limit}.
\end{proof}

%%------------------------------------------------------------------------------------------------------------------------------------------------------------------------------------------------------------%%
%%------------------------------------------------------------------------------------------------------------------------------------------------------------------------------------------------------------%%
\begin{lemma}\label{eq sq fdb}
For all $r \ge 0$ there is a constant $C_r > 0$ such that 
$$
\sup_{|q| \le 1} \norm{e^{q\cdot}s_q}_{W^{r,\infty}} \le C_r.
$$
\end{lemma}

\begin{proof}
Set $f(x) = e^x$, $N(X) = X^{-1}$, and $g(x) = (e^x+e^{-x})/2$, so
\begin{align*}
\partial_x^r[e^{x}s_1(x)]
&= \partial_x^r[f(x)N(g(x))] \\
\\
&= \sum_{k=0}^r{r \choose k} \partial_x^{r-k}[f]\partial_X^k[N(g)] \\
\\
&= \sum_{k=0}^r{r\choose k} \partial_x^{r-k}[f]\sum_{j=1}^k\partial_X^j[N](g)\sum_{\sigmab \in \Sigma_j^k}C_{\sigmab}\prod_{\ell=1}^j \partial_x^{\sigma_j}[g] \\
\\
&= \sum_{k=0}^r {r \choose k} e^x\sum_{j=1}^k (-1)^jj!\left(\frac{e^x+e^{-x}}{2}\right)^{-(j+1)}\sum_{\sigmab \in \Sigma_j^k}C_{\sigmab}\prod_{\ell=1}^j\frac{e^x+(-1)^{\sigma_j}e^{-x}}{2}.
\end{align*}
The $k$th term of this sum is bounded by
$$
\frac{1}{2^{j+1}}{r \choose k}\frac{e^x}{(e^x+e^{-x})^{j+1}}\sum_{\sigmab \in \Sigma_j^k}C_{\sigmab} \frac{(e^x+e^{-x})^j}{2^j}
= C_r\frac{e^x}{e^x+e^{-x}},
$$
and we know that 
$$
\sup_{X > 0} \frac{X}{X+X^{-1}} = \sup_{X >0 } \frac{X^2}{X^2+1} = 1.
$$
\end{proof}

%%------------------------------------------------------------------------------------------------------------------------------------------------------------------------------------------------------------%%
%%------------------------------------------------------------------------------------------------------------------------------------------------------------------------------------------------------------%%
%%------------------------------------------------------------------------------------------------------------------------------------------------------------------------------------------------------------%%
\subsubsection{The Friesecke-Pego operator}
Our goal in this section is to prove --- from scratch --- that the operator 
$$
\A{f} 
:= f + \bunderbrace{\frac{2\kappa}{\kappa+1}\left(\frac{\beta}{\kappa^3}+1\right)\varpi^0(\sigma{f})}{-\K{f}}, 
\qquad
\varpi^0 = -c_{\kappa}^2(1-\alpha_{\kappa}\partial_X^2)^{-1},
$$
is invertible on $E_q^r$. Our method follows exactly the proof in \cite{friesecke-pego1} for a differently scaled version of $\A$.  

To see that $\A$ maps $E^r$ to $E^r$ for arbitrary $r \ge 1$, fix $f \in E^r$.  Then $\sigma{f} \in E^r$ since $\sigma \in W^{r,\infty}$ is even.  Then $\varpi^0(\sigma{f}) \in E^r$ since $\varpi^0$ smooths by two and has an even symbol.  Hence $\A{f} = f -\K{f} \in E^r$.  

We will control the kernel of $\A$ with the following lemma.

%%------------------------------------------------------------------------------------------------------------------------------------------------------------------------------------------------------------%%
%%------------------------------------------------------------------------------------------------------------------------------------------------------------------------------------------------------------%%
\begin{lemma}
\label{ode lemma from Doug}
Let $\lambda > 0$ and $\varsigma \in \C_0(\R)$. Then the second-order differential equation
\begin{equation}
\label{ode-eig}
\psi''(t)+\lambda(\varsigma(t)-1)\psi(t) = 0, \ t \in [0,\infty)
\end{equation}
does not have two linearly independent bounded solutions. 
\end{lemma}

\begin{proof}
Supposfe instead that \eqref{ode-eig} has two bounded, linearly independent solutions $f_1$ and $f_2$.  Since the coefficients of \eqref{ode-eig} are continuous, there exist scalars $\alpha_1,\alpha_2$ such that $f := \alpha_1f_1+\alpha_2f_2$ solves 
\begin{equation}\label{contrived ode}
\begin{cases}
f''(t) + \lambda(\varsigma(t)-1)f(t) = 0,  &t \in [0,\infty) \\
f(t_0) = f'(t_0) = 1,
\end{cases}
\end{equation}
where by the hypothesis on $\varsigma$, we have chosen $t_0 \ge 0$ such that if $t \ge t_0$, then $|\varsigma(t)| < {1}/{2}$.  \timcomment{Cite/find source for this ODE fact.}

Let
$$
\mathcal{S} 
= \set{t > t_0}{f(s) > 0 \ \forall s \in (t_0,t)}.
$$
Since $f(t_0) = 1$, by continuity $\mathcal{S}$ is nonempty, and so $T := \sup(\mathcal{S}) \in (t_0,\infty]$.  We first show that $(t_0,T) \subseteq \mathcal{S}$ and then that $T = \infty$.  

For the first claim, let $t \in (t_0,T)$. Then there must exist $t_1 \in \mathcal{S}$ such that $t < t_1$, as otherwise $T \le t$.  So, $t \in (t_0,t_1)$, where $f(s) > 0$ for all $s \in (t_0,t_1)$.  Hence $f(s) > 0$ for all $s \in (t_0,t] \subseteq (t_0,t_1)$, and so $t \in \mathcal{S}$.  In particular, note that $f(t) > 0$ for all $t \in (t_0,T)$.  

For the second claim, let $t \in (t_0,T)$ and compute
$$
f''(t) 
= \lambda(1-\varsigma(t))f(t)
\ge \lambda{f}(t)-\lambda\frac{f(t)}{2} = \lambda\frac{f(t)}{2} > 0.
$$
Hence $f'$ is increasing on $(t_0,\infty)$, and so, using the initial conditions of \eqref{contrived ode}
\begin{equation}\label{ftc contradiction}
f(t) 
= f(t_0) + \int_{t_0}^t f'(s)\ds 
\ge f(t_0) + f'(t_0)(t-t_0) 
= 1+t-t_0.
\end{equation}
Then
$$
f(T) 
= \lim_{t \to T^-} f(t) \ge \lim_{t \to T^-} 1+t-t_0 
= 1+T-t_0 
> 0.
$$
By continuity, there is $\delta > 0$ such that $f(t) > 0$ for $t \in [T,T+\delta)$. Hence $T + \delta \in \mathcal{S}$, which is a contradiction unless $T = \infty$. 

So, we have $\mathcal{S} = (t_0,\infty)$, and therefore $f(t) > 0$ for all $t \in (t_0,\infty)$.  But then \eqref{ftc contradiction} holds for all $t > t_0$, and so $f$ is unbounded, a contradiction.
\end{proof}

Now suppose $\A{f} = 0$, $f \in L^2$.  That is,
\begin{equation}\label{ker A equation}
f -\frac{2\kappa}{\kappa+1}\left(\frac{\beta}{\kappa^3}+1\right)c_{\kappa}^2(1-\alpha_{\kappa}\partial_X^2)^{-1}(\sigma{f}) = 0.
\end{equation}
It is straightforward to rearrange this to
\begin{equation}\label{ker A rearranged}
f'' + \frac{1}{\alpha_{\kappa}}\left(\frac{2\kappa}{\kappa+1}\left(\frac{\beta}{\kappa^3}+1\right)c_{\kappa}^2\sigma-1\right)f = 0,
\end{equation}
and then Lemma \eqref{ode lemma from Doug} applies to show that \eqref{ker A rearranged} has at most one nontrivial bounded solution. Since \eqref{ker A equation} and \eqref{ker A rearranged} are equivalent, the dimension of the kernel of $\A$ (as an operator from $H^r$ to $H^r$) is at most one.  Now we show the dimension is precisely one.

We know that $\sigma$ solves the KdV-type equation
$$
\sigma-\frac{1}{2}\K\sigma
= \sigma - c_{\kappa}^2(1-\alpha_{\kappa}\partial_X^2)^{-1}\left(\frac{\kappa}{\kappa+1}\left(\frac{\beta}{\kappa^3}+1\right)\sigma^2\right) 
= 0.
$$
Then since derivatives commute with Fourier multipliers,
\begin{align*}
\A\sigma'
&= \sigma'-\left(\frac{2\kappa}{\kappa+1}\left(\frac{\beta}{\kappa^3}+1\right)\sigma\sigma'\right) \\
\\
&= \sigma' - \frac{\kappa}{\kappa+1}\left(\frac{\beta}{\kappa^3}+1\right)(1-\alpha_{\kappa}\partial_X^2)^{-1}(2\sigma\sigma') \\
\\
&= \partial_X[\sigma]-\frac{\kappa}{\kappa+1}\left(\frac{\beta}{\kappa^3}+1\right)(1-\alpha_{\kappa}\partial_X^2)^{-1}(\partial_X[\sigma^2]) \\
\\
&= \partial_X\left(\sigma-\frac{1}{2}\K\sigma\right) \\
\\
&= 0.
\end{align*}
That is, $\ker(\A) = \spn(\{\sigma'\})$. Since $\sigma$ is even, $\sigma'$ is odd, and so if we restrict $\A$ to $L^2 \cap \{even functions\}$, then $\ker(\A)$ is trivial.  In particular, $\restr{\A}{E^r}$ has trivial kernel.  

Since $\A = \ind - \K$, where $\K$ is compact, the Fredholm alternative guarantees that $\restr{\A}{E^r}$ is also surjective, hence $\restr{\A}{E^r}$ is invertible.

%%------------------------------------------------------------------------------------------------------------------------------------------------------------------------------------------------------------%%
%%------------------------------------------------------------------------------------------------------------------------------------------------------------------------------------------------------------%%
\begin{proposition}\label{fp extension}
There exists $q_{\sf{FP}} > 0$ such that for $q \in (0,q_{\sf{FP}})$ the operator $\A$ maps $E_q^r$ bijectively onto $E_q^r$.
\end{proposition}

\begin{proof}
Recall that the symbol of $\varpi^0$ is 
$$
\tvarpi^0(k) := \tilde{\varpi^0}(k) = \frac{1}{1+\alpha_{\kappa}k^2},
$$
where $\alpha_{\kappa} > 0$.  Then $\tvarpi^0$ has no singularities whatsoever in the strip $\Sigma_{\sqrt{\alpha_{\kappa}}}$, and clearly the other hypotheses of Beale's lemma apply to it.  Hence $\varpi^0$ maps $H_q^r$ into $H_q^r$ for $q \in (0,\sqrt{\alpha_{\kappa}})$, and since $\tvarpi^0$ is even, this restricts further to map $E_q^r$ into $E_q^r$.  Since $\sigma$ is even and $\sigma \in H_q^r$ for all $r \ge 0$ and all $q \in (0,1/2\sqrt{\alpha_{\kappa}})$, multiplication by $\sigma$ maps $E_q^r$ to $E_q^r$ (Lemma \ref{Hrq multiplication operator}), so the composition $\varpi^0(\sigma\cdot)$ also maps $E_q^r$ into $E_q^r$. Hence $\A \in \b(E_q^r,E_q^r)$.

It remains for us to show that $\A$ is bijective from $E_q^r$ to $E_q^r$.  We provide two proofs.

%%------------------------------------------------------------------------------------------------------------------------------------------------------------------------------------------------------------%%
%%------------------------------------------------------------------------------------------------------------------------------------------------------------------------------------------------------------%%
\begin{enumerate}[label={\bf(\roman*)}]
%%------------------------------------------------------------------------------------------------------------------------------------------------------------------------------------------------------------%%
\item One easy way to do this is to note first that $\A$ has trivial kernel on $E_q^r$: by the discussion above, $\A$ has trivial kernel on $E^r$, and $E_q^r \subseteq E^r$.  Next, we note that Corollary \ref{Hrq compact operator corollary} implies that $\K$ is compact from $E_q^r$ to $E_q^r$.  The Fredholm alternative applies (once again) to show that $\A$ is invertible on $E_q^r$.  

%%------------------------------------------------------------------------------------------------------------------------------------------------------------------------------------------------------------%%
\item A longer proof illustrates the method of operator conjugation.  Let 
$$
\A_qf 
:= c_q\A(s_qf)
= f - c_q\K(s_qf).
$$
First we show that $\A_q \in \b(E^r,E^r)$.  Beale's lemma tells us that if $f \in E^r$, then $s_qf \in E_q^r$, so $\K(s_qf) \in E_q^r$ as well, and then $c_q\K(s_qf) \in E^r$.  So, $\A_q$ maps $E^r$ to $E^r$.  For its boundedness, we only need to estimate
$$
\norm{c_q\K(s_qf)}_{E^r}
= \norm{\K(s_qf)}_{E_q^r}
\le \norm{\K}_{\b(E_q^r,E_q^r)}\norm{s_qf}_{E_q^r}
= \norm{\K}_{\b(E_q^r,E_q^r)}\norm{f}_{E^r}.
$$

Next, we show that $\A$ is invertible on $E_q^r$ if and only if $\A_q$ is invertible on $E^r$.  This is due to the equivalences
$$
\A{f} = g
\iff
\A(s_q\tilde{f}) = s_q\tilde{g}
\iff
c_q\A(s_q\tilde{f}) = \tilde{g}
\iff
\A_q\tilde{f} = \tilde{g}
$$ 
and
$$
\A{f} = \A{g}
\iff
c_q\A(s_q\tilde{f}) = c_q\A(s_q\tilde{g})
\iff 
\A_q\tilde{f} = \A_q\tilde{g}
$$
for $f = s_q\tilde{f}$, $g = s_q\tilde{g} \in E_q^r$ and $\tilde{f}$, $\tilde{g} \in E^r$.

Finally, we compute
$$
\frac{1}{1+(k+iq)^2}-\frac{1}{1+k^2}
= \bunderbrace{\frac{q^2(1-3k^2-q^2)}{(k^2+1)((k^2-q^2+1)^2+(2kq)^2}}{\rhs_q(k)}-i\bunderbrace{\frac{2kq}{(k^2-q^2+1)^2+(2kq)^2}}{\I_q(k)}.
$$
If we restrict $q \in (0,1/2)$, then
$$
\left(\frac{3}{4}+k^2\right)^2 
\le (k^2-q^2+1)^2+(2kq)^2,
$$
in which case
$$
|\rhs_q(k)| 
\le |q|\frac{|1-3k^2|}{(3/4+k^2)^2}+
\frac{|q|}{4}\frac{1}{(3/4+k^2)^2}
\le 4|q|
$$
and
$$
|\I_q(k)|
\le |q|\left|\frac{2k}{(3/4+k^2)^2}\right|
\le 2|q|.
$$
So, we may use operator conjugation to establish
$$
\norm{\A_q-\A}_{\b(E^r,E^r)}
= \norm{\K_q-\K}_{\b(E^r,E^r)}
\to 0
$$
as $q \to 0$. Since $\A$ is invertible, this shows that for $q$ sufficiently small $\A_q$ is invertible as well. \qedhere
\end{enumerate} 
\end{proof}
