# Supplementary material for: Nanopteron-stegoton traveling waves in spring dimer Fermi-Pasta-Ulam-Tsingou lattices
Source: arXiv:1710.07376 source file (2017-10-20)
Supplement: Supplementary file 2 [file appendix_sobolev_spaces_compact_embedding.tex]

%%------------------------------------------------------------------------------------------------------------------------------------------------------------------------------------------------------------%%
%%------------------------------------------------------------------------------------------------------------------------------------------------------------------------------------------------------------%%
%%------------------------------------------------------------------------------------------------------------------------------------------------------------------------------------------------------------%%
\subsubsection{The compact embedding of $H_q^r$ into $H_q^{r-1}$} 
For these proofs it will be convenient to norm $H_q^r$ with 
$$
\norm{f}_{r,q} = \norm{\cosh^q(\cdot)f}_{H^r}.
$$

%%------------------------------------------------------------------------------------------------------------------------------------------------------------------------------------------------------------%%
%%------------------------------------------------------------------------------------------------------------------------------------------------------------------------------------------------------------%%
\begin{lemma}\label{Hrq multiplication operator lemma}
Let $\varsigma \in H_q^r$.  There exists a constant $C > 0$ such that 
\begin{equation}\label{Hrq multiplication operator}
\norm{\varsigma{f}}_{r,q} \le C\norm{f}_{H^r}
\end{equation}
for all $f \in H^r$.
\end{lemma}

\begin{proof}
Recall the inequality
$$
|\cosh^b(X)\varsigma(X)|
\le \norm{\cosh^b(\cdot)\varsigma}_{L^{\infty}}
\le C_{r,b}\norm{\varsigma}_{r,b} 
\Longrightarrow 
|\varsigma(X)| \le C_{r,b}\sech^b(X).
$$
Then
$$
\norm{\varsigma{f}}_{r,q+b} = \norm{\cosh^{q+b}(\cdot)\varsigma{f}}_{L^2} + \norm{\cosh^{q+b}(\cdot)\partial_X^r[\varsigma{f}]}_{L^2},
$$
where
\begin{equation}\label{mult op 1}
\norm{\cosh^{q+b}(\cdot)\varsigma{f}}_{L^2} \le \norm{\cosh^b(\cdot)\varsigma}_{L^{\infty}}\norm{\cosh^q(\cdot)f}_{L^2} 
\end{equation}
and
$$
\norm{\cosh^{q+b}(\cdot)\partial_X^r[\varsigma{f}]}_{L^2}
\le C_{r,q+b}\sum_{k=0}^r \norm{\cosh^{q+b}(\cdot)\partial_X^k[\varsigma]\partial_X^{r-k}[f]}_{L^2}.
$$
Here we have used \eqref{coshq ineq}.  When $k = 0$, we have
\begin{equation}\label{mult op 2}
\norm{\cosh^{q+b}(\cdot)\varsigma\partial_X^r[f]}_{L^2}
\le \norm{\cosh^b(\cdot)\varsigma}_{L^{\infty}}\norm{\cosh^q(\cdot)\partial_X^r[f]}_{L^2}
\end{equation}
and for $1 \le k \le r$, 
\begin{equation}\label{mult op 3}
\norm{\cosh^{q+b}(\cdot)\partial_X^k[\varsigma]\partial_X^{r-k}[f]}_{L^2}
\le \norm{\cosh^q(\cdot)\partial_X^{r-k}[f]}_{L^{\infty}}\norm{\cosh^b(\cdot)\partial_X^k[\varsigma]}_{L^2}.
\end{equation}
Combining \eqref{mult op 1}, \eqref{mult op 2}, and \eqref{mult op 3}, we arrive at the bound \eqref{Hrq multiplication operator}.  
\end{proof}

%%------------------------------------------------------------------------------------------------------------------------------------------------------------------------------------------------------------%%
%%------------------------------------------------------------------------------------------------------------------------------------------------------------------------------------------------------------%%
\begin{lemma}\label{base case Hrq compact embedding}
Let $b$, $q > 0$.  The space $H_{q+b}^1$ is compactly embedded in $L_q^2$.
\end{lemma}

\begin{proof}
Let $(f_n)$ be a bounded sequence in $H_{q+b}^1$, so $(f_n)$ is a bounded sequence in $H^1$ with
$$
M 
:= \sup_{n \in \N} \norm{f_n}_{H_{q+b}^1} 
< \infty.
$$
Note that
\begin{equation}\label{general sech bound}
\begin{aligned}
|f_n(x)| 
&= \sech^{q+b}(x)|\cosh^{q+b}(x)f_n(x)| \\
\\
&\le \sech^{q+b}(x)\norm{\cosh^{q+b}(\cdot)f_n}_{L^{\infty}} \\
\\
&\le C\sech^{q+b}(x)\norm{f_n}_{H_{q+b}^1} \\
\\
&\le C_{\star}\sech^{q+b}(x), \ C_{\star} := CM.
\end{aligned}
\end{equation}

For $N \in \N$, since $H^1([-N,N])$ embeds compactly into $L^2([-N,N])$, there exists a subsequence $(f_{\varphi_N(n)})$ of $(f_n)$ such that $(f_{\varphi_N(n)})$ converges to some function $F_{(N)}$ in $L^2([-N,N])$.  Each map $\varphi_N \colon \N \to \N$ is necessarily strictly increasing.  We may select this subsequence inductively so that $(f_{\varphi_{N+1}(n)})$ is a subsequence of $(f_{\varphi_N(n)})$ and so that $(f_{\varphi_N(n)})$ also converges pointwise a.e. on $[-N,N]$ to $F_{(N)}$.  (For the pointwise convergence, we recall Theorem VII.1.4 in \cite{lang}.) We observe several properties of $F_{(N)}$.

\begin{itemize}
%%------------------------------------------------------------------------------------------------------------------------------------------------------------------------------------------------------------%%
\item Since $(f_{\varphi_{N+1}(n)})$ is a subsequence of $(f_{\varphi_N(n)})$, we have $F_{(N+1)} = F_{(N)}$ on $[-N,N]$.
%%------------------------------------------------------------------------------------------------------------------------------------------------------------------------------------------------------------%%
\item The pointwise convergence on $[-N,N]$ combines with \eqref{general sech bound} to produce
\begin{equation}\label{FN sech bound}
|F_{(N)}(x)| = \lim_{n \to \infty} |f_{\varphi_N(n)}(x)| \le C_{\star}\sech^{q+b}(x)
\end{equation}
a.e. on $[-N,N]$.  
%%------------------------------------------------------------------------------------------------------------------------------------------------------------------------------------------------------------%%
\item Since $\cosh(b\cdot)$ is bounded on $[-N,N]$, the Cauchy-Schwarz inequality leads us to an integer $\psi(N)$ large enough that if $n \ge \psi(N)$, then
\begin{equation}\label{diagonal estimate}
\norm{\cosh^q(\cdot)(f_{\varphi_N(n)} - F_{(N)})}_{L^2([-N,N])} < \frac{1}{\sqrt{N}}.
\end{equation}
We may take $\psi(N) < \psi(N+1)$ for each $N$.  Let $\Phi(N) = \varphi_N(\psi(N))$.  Since $\psi$ is strictly increasing on $\N$, it is easy to see that $\Phi$ is also strictly increasing:
\begin{align*}
\Phi(N+1) &= \varphi_{N+1}(\psi(N+1)) \\
\\
&> \varphi_{N+1}(\psi(N)) \text{ because } \psi(N) < \psi(N+1) \text{ and } \varphi_{N+1} \text{ is strictly increasing} \\
\\
&\ge \varphi_N(\psi(N))
\end{align*}
because $(f_{\varphi_{N+1}}(n))$ is a subsequence\footnote{
In the language of our proof above, we fix $N \in \N$ and take $\lambda(n) = f_{\varphi_N(n)}$ and $\mu(n) = f_{\varphi_{N+1}(n)}$. Then there is a strictly increasing function $\iota \colon \N \to \N$ such that $\mu(n) = \lambda(\iota(n))$, i.e., $f_{\varphi_{N+1}(n)} = f_{\varphi_N(\iota(n))}$.  Hence $\varphi_{N+1}(n) = \varphi_N(\iota(n)) \ge \varphi_N(n)$.
} 
of $(f_{\varphi_N(n)})$. Thus $(f_{\Phi(N)})$ is a subsequence of $(f_n)$.
\end{itemize}

Now let $f(x) = F_{(N)}(x)$ when $|x| \le N$.  (Another formula for $f$ is $f(x) = F_{(|\lceil{x}\rceil|)}(x).$)  We see from \eqref{FN sech bound} that 
\begin{equation}\label{estimate on f}
|f(x)| \le C_{\star}\sech^{q+b}(x)
\end{equation}
a.e. on $\R$.  If we know that $f$ is measurable, then we will have $\cosh^q(\cdot)f \in L^2$ from this inequality.  Given $E \subseteq \R$ measurable, we have
$$
f^{-1}(E) = \bigcup_{N=1}^{\infty} f^{-1}(E \cap [-N,N]) = \bigcup_{N=1}^{\infty} F_{(N)}^{-1}(E \cap [-N,N]).
$$
Each set $F_{(N)}^{-1}(E \cap [-N,N])$ is measurable since $F_{(N)} \in L^2([-N,N])$.  And so $f$ is measurable. Hence $f \in L_b^2$.

Now we can show that
\begin{equation}\label{Hrq compact embedding limit}
\lim_{N \to \infty} \norm{f_{\Phi(N)} - f}_{L_b^2} = 0.
\end{equation}
Let $\ep > 0$ and take $N_{\ep} \in \N$ so large that 
$$
\max\left\{\frac{1}{N_{\ep}}, 8C_{\star}^2\int_{N_{\ep}}^{\infty} \sech^{2b}(x) \dx\right\} < \frac{\ep}{2}.
$$
Then for $N \ge N_{\ep}$, we have
\begin{align*}
\norm{\cosh^q(\cdot)(f_{\Phi(N)}-f)}_{L^2}^2 
&= \int_{-\infty}^{-N} \cosh^{2q}(x)|f_{\Phi(N)}(x)-f(x)|^2 \dx \\
&+ \int_{-N}^N \cosh^{2q}(x)|f_{\Phi(N)}(x)-f(x)|^2 \dx \\
&+ \int_N^{\infty} \cosh^{2q}(x)|f_{\Phi(N)}(x)-f(x)|^2\dx.
\end{align*}
We estimate the second integral using \eqref{diagonal estimate}:
\begin{equation}\label{middle integral estimate}
\int_{-N}^N \cosh^{2q}(x)|f_{\Phi(N)}(x)-f(x)|^2 \dx = \norm{\cosh^q(\cdot)(f_{\Phi(N)}-f)}_{L^2([-N,N]}^2 < \frac{1}{N} \le \frac{1}{N_{\ep}} < \frac{\ep}{2}.
\end{equation}
For the first and third integrals, we use \eqref{general sech bound} and \eqref{estimate on f}:
\begin{align*}
\cosh^{2q}(x)|f_{\Phi(N)}(x)-f(x)|^2 
&\le \cosh^{2q}(x)|f_{\Phi(N)}(x)|^2 + 2\cosh^{2q}(x)|f_{\Phi(N)}(x)||f(x)| \\
&+ \cosh^{2q}(x)|f(x)|^2 \\
\\
&\le C_{\star}^2\cosh^{2q}(x)\sech^{2q+2b}(x)+2C_{\star}^2\cosh^{2q}\sech^{2q+2b}(x)\\
&+C_{\star}^2\cosh^{2q}(x)\sech^{2q+2b}(x) \\
\\
&= 4C_{\star}^2\sech^{2b}(x).
\end{align*}
Thus
\begin{multline}\label{outer integrals estimate}
\int_{-\infty}^{-N} \cosh^{2b}(x)|f_{\Phi(N)}(x)-f(x)|^2 \dx + \int_N^{\infty} \cosh^{2b}(x)|f_{\Phi(N)}(x)-f(x)|^2\dx \\
\le 4C_{\star}^2\int_{-\infty}^{-N}\sech^{2\ep}(x) \dx + 4C_{\star}^2\int_{N}^{\infty} \sech^{2\ep}(x) \dx 
= 8C_{\star}^2\int_N^{\infty} \sech^{2b}(x) \dx 
< \frac{\ep}{2}.
\end{multline}
We combine this with \eqref{middle integral estimate} to conclude that $N \ge N_{\ep}$, we have
$$
\norm{\cosh^q(\cdot)(f_{\Phi(N)}-f)}_{L^2}^2 < \ep,
$$
and so the limit \eqref{Hrq compact embedding limit} holds.
\end{proof}

%%------------------------------------------------------------------------------------------------------------------------------------------------------------------------------------------------------------%%
%%------------------------------------------------------------------------------------------------------------------------------------------------------------------------------------------------------------%%
\begin{lemma}\label{weak derivative convergence lemma}
Let $d \ge 1$, $U \subseteq \R^d$ be open and $f \in H_q^r(U)$ for $q \ge 0$. Let $(f_n)$ be a sequence in $H_q^r$ such that $f_n \to f$ in $L_q^2$ and $D^{\alphab}[f_n] \to g_{\alphab}$ in $L_q^2$ for some $0 < |\alphab| \le r$ and some $g_{\alphab} \in L_q^2(U)$.  Then $g_{\alphab} = D^{\alphab}[f]$.
\end{lemma}

\begin{proof}
Let $\varphi \in C_c^{\infty}(U)$.  Then
$$
\int_U \varphi(D^{\alphab}[f]-g_{\alphab})
= \bunderbrace{\int_U \varphi(D^{\alphab}[f]-D^{\alphab}[f_n])}{\mathcal{I}_1} + \bunderbrace{\int_U \varphi(D^{\alphab}[f_n]-g_{\alphab})}{\mathcal{I}_2}.
$$
The definition of the weak derivative gives
$$
\int_U\varphi D^{\alphab}[f] = (-1)^{|\alphab|}\int_U D^{\alphab}[\varphi]f_n \quadword{and} \int_U\varphi D^{\alphab}[f_n] = (-1)^{|\alphab|}\int_U D^{\alphab}[\varphi] f_n.
$$
Hence
$$
\mathcal{I}_1 = (-1)^{|\alphab|} \int_U D^{\alphab}[\varphi](f-f_n),
$$
and so, using the Cauchy-Schwarz inequality,
\begin{align*}
\left|\int_U\varphi (D^{\alphab}[f]-g_{\alphab}) \right|
&\le |\mathcal{I}_1| + |\mathcal{I}_2| \\
\\
&\le \norm{D^{\alphab}[\varphi]}_{L^2}\norm{f_n-f}_{L^2} + \norm{\varphi}_{L^2}\norm{D^{\alphab}[f_n]-g_{\alphab}}_{L^2} \\
\\
&\le \norm{D^{\alphab}[\varphi]}_{L^2}\norm{f_n-f}_{L_q^2} + \norm{\varphi}_{L^2}\norm{D^{\alphab}[f_n]-g_{\alphab}}_{L_q^2}.
\end{align*}
Thus
$$
\int_U\varphi (D^{\alphab}[f]-g_{\alphab}) = 0
$$
for all $\varphi \in C_c^{\infty}(U)$, and so $D^{\alphab}[f] = g_{\alphab}$.
\end{proof}

%%------------------------------------------------------------------------------------------------------------------------------------------------------------------------------------------------------------%%
%%------------------------------------------------------------------------------------------------------------------------------------------------------------------------------------------------------------%%
\begin{proposition}\label{Hrq compact embedding prop}
Let $b > 0$, $q \ge 0$ and $r \in \N$.  Then $H_{q+b}^{r+1}$ is compactly embedded in $H_q^r$ (where $H_0^r = H^r$).
\end{proposition}

\begin{proof}
We have proved the $r = 0$ case in Lemma \ref{base case Hrq compact embedding} and so we induct on $r$.  If the proposition is true for $k=0,\ldots,r$ and $(f_n)$ is a bounded sequence in $H_{q+b}^{r+1}$, then $(\partial_X^k[f_n])$ is bounded in $H_{q+b}^1$ for $k = 0,\ldots,r$, and so, passing to subsequences and relabeling as needed, there exist a subsequence $(f_{n_j})$ of $(f_n)$ and functions $g_0,\ldots,g_r \in L_q^2$ such that $\partial_X^k[f_{n_j}] \to g_k$ in $L_q^2$.  By Lemma \ref{weak derivative convergence lemma}, we have $g_k = \partial_X^k[g_0]$.  That is, 
$$
\lim_{j \to \infty} \norm{f_{n_j}-g_0}_{H_q^r} 
= \lim_{j \to \infty} \sum_{k=0}^r \norm{\partial_X^k[f_{n_j}-g_0]}_{L_q^2} 
=0,
$$
and so $f_{n_j} \to g_0$ in $H_q^r$.
\end{proof}

It will be useful to know that a certain composition of smoothing and multiplication operators is compact when the multiplication induces decay.

%%------------------------------------------------------------------------------------------------------------------------------------------------------------------------------------------------------------%%
%%------------------------------------------------------------------------------------------------------------------------------------------------------------------------------------------------------------%%
\begin{corollary}\label{Hrq compact operator corollary}
Let $b > 0$, $q \ge 0$, $\varpi \in \b(H_q^{r-1},H_q^r)$, and $\varsigma \in H_b^r$.  The operator $f \mapsto \varpi(\varsigma{f})$ is compact from $H_q^r$ to $H_q^r$.
\end{corollary}

\begin{proof}
The following diagram summarizes the proof.
$$
H_q^r 
\xrightarrow{f \mapsto \varsigma{f}} 
H_{q+b}^r
\xhookrightarrow{\varsigma{f} \mapsto \varsigma{f}}
H_q^{r-1}
\xrightarrow{\varsigma{f} \mapsto \varpi(\varsigma{f})} 
H_q^r
$$
By Lemma \ref{Hrq multiplication operator lemma}, we know that $f \mapsto \varsigma{f}$ is a bounded operator from $H_q^r$ to $H_{q+b}^r$.  Then Proposition \ref{Hrq compact embedding prop} implies that the identity mapping $\varsigma{f} \mapsto \varsigma{f}$ is compact from $H_{q+b}^r$ to $H_q^{r-1}$.  Hence $f \mapsto \varpi(\varsigma{f})$ is also compact from $H_q^r$ to $H_q^r$.
\end{proof}
