# Supplementary material for: Nanopteron-stegoton traveling waves in spring dimer Fermi-Pasta-Ulam-Tsingou lattices
Source: arXiv:1710.07376 source file (2017-10-20)
Supplement: Supplementary file 3 [file appendix_sobolev_spaces_equivalences.tex]

%%------------------------------------------------------------------------------------------------------------------------------------------------------------------------------------------------------------%%
%%------------------------------------------------------------------------------------------------------------------------------------------------------------------------------------------------------------%%
%%------------------------------------------------------------------------------------------------------------------------------------------------------------------------------------------------------------%%
\subsubsection{Equivalent definitions of some weighted Sobolev spaces}

\timcomment{This section can be eliminated with just the definition of $\norm{f}_{r,q} := \norm{\cosh(q\cdot)f}_{L^2} + \norm{\cosh(q\cdot)\partial_X^r[f]}_{L^2}$ kept in.}
Let 
$$
\X_q^r = \set{f \in H^r}{\cosh(q\cdot)f \in H^r}
$$
$$
\Y_q^r = \set{f \in H^r}{\cosh^q(\cdot)f \in H^r}
$$
$$
\norm{f}_{\X_q^r} = \norm{\cosh(q\cdot)f}_{H^r}
$$
$$
\norm{f}_{\Y_q^r} = \norm{\cosh^q(\cdot)f}_{H^r}
$$
$$
\triplenorm{f}_{\X_q^r} = \norm{\cosh(q\cdot)f}_{L^2} + \norm{\cosh(q\cdot)\partial_X^r[f]}_{L^2}
$$
$$
\triplenorm{f}_{\Y_q^r} = \norm{\cosh^q(\cdot)f}_{L^2} + \norm{\cosh^q(\cdot)\partial_X^r[f]}_{L^2}
$$
These distinctions are seemingly trivial, as the following result indicates.  However, to estimate the norms of certain functions, it is convenient to switch back and forth among the four norms above.  

%%------------------------------------------------------------------------------------------------------------------------------------------------------------------------------------------------------------%%
%%------------------------------------------------------------------------------------------------------------------------------------------------------------------------------------------------------------%%
\begin{theorem}\label{weighted equiv theorem}
$\X_q^r = \Y_q^r$ and the norms $\norm{\cdot}_{\X_q^r}$, $\norm{\cdot}_{\Y_q^r}$, $\triplenorm{\cdot}_{\X_q^r}$, and $\triplenorm{\cdot}_{\Y_q^r}$ are all equivalent. 
\end{theorem}

We prove this theorem in Lemmas \ref{Xrq norm equivalence}, \ref{Yrq equivalence lemma}, and \ref{cosh equiv lemma}.
%\ref{Xrq lemma}, \ref{Yrq lemma}, and \ref{cosh equiv lemma} 
below.  
We write 
$$
H_q^r = \X_q^r = \Y_q^r.
$$
We use whichever of the four norms $\norm{\cdot}_{\X_q^r}$, $\norm{\cdot}_{\Y_q^r}$, $\triplenorm{\cdot}_{\X_q^r}$, and $\triplenorm{\cdot}_{\Y_q^r}$ we find convenient and denote this norm by
$$
\norm{f}_{H_q^r} = \norm{f}_{r,q}.
$$

%%------------------------------------------------------------------------------------------------------------------------------------------------------------------------------------------------------------%%
%%------------------------------------------------------------------------------------------------------------------------------------------------------------------------------------------------------------%%
\begin{lemma}\label{Xrq norm equivalence}
The norms $\norm{\cdot}_{\X_q^r}$ and $\triplenorm{\cdot}_{\X_q^r}$ are equivalent on $H_q^r$.
\end{lemma}

\begin{proof}
Lemma \ref{lemma for q ft deriv} shows that if $f \in H_q^r$, then $\cosh(q\cdot)\partial_X^r[f] \in L^2$, so $\triplenorm{\cdot}_{\X_q^r}$ is indeed defined on $H_q^r$.  

First we show there is $C_{r,q} > 0$ such that 
$$
\norm{f}_{\X_q^r} \le C_{r,q}\triplenorm{f}_{\X_q^r}, \ f \in \X_q^r.
$$
We have
$$
\norm{\partial_X^r[c\cosh(q\cdot)_qf]}_{L^2} = \norm{\hat{\partial_X^r[\cosh(q\cdot)f]}}_{L^2}
$$
and
\begin{align*}
\hat{\partial_X^r[\cosh(q\cdot)f]}(k)
&= (ik)^r\hat{\cosh(q\cdot)f}(k) \\
\\
&= (ik)^r\frac{\hat{f}(k+iq)+\hat{f}(k-iq)}{2} \\
\\
&= (ik-q+q)^r\frac{\hat{f}(k+iq)}{2}+(ik+q-q)\frac{\hat{f}(k-iq)}{2} \\
\\
&= \sum_{j=0}^r {r \choose j} (ik-q)^jq^{r-j}\frac{\hat{f}(k+iq)}{2}
+ \sum_{j=0}^r {r \choose j} (ik+q)^j(-q)^{r-j}\frac{\hat{f}(k-iq)}{2} \\
\\
&= \sum_{j=0}^r {r \choose j}q^{r-j}\left(
(i(k+iq))^j\frac{\hat{f}(k+iq)}{2}
+ (-1)^{r-j}(i(k-iq))^j\frac{\hat{f}(k-iq)}{2}
\right).
\end{align*}
Using \eqref{j r domination}, we find
\begin{align*}
\left|(k\pm{i}q)^j\frac{\hat{f}(k\pm{iq})}{2}\right|
&\le \frac{|\hat{f}(k\pm iq)|}{2}
+ \frac{|(k\pm iq)^r\hat{f}(k \pm iq)|}{2} \\
\\
&= \frac{|\hat{e^{\pm q\cdot}f}(k)|}{2}
+ \frac{|\hat{\partial_X^r[f]}(k \pm iq)|}{2} \\
\\
&=\frac{|\hat{e^{\pm q\cdot}f}(k)|}{2}
+ \frac{|\hat{e^{\pm q}\partial_X^r[f]}(k)|}{2},
\end{align*}
and so 
\begin{align*}
\norm{\partial_X^r[\cosh(q\cdot)f]}_{L^2}
&\le C_{r,q}\left(\norm{\hat{e^{q\cdot}f}}_{L^2}
\norm{\hat{e^{-q\cdot}f}}_{L^2}
+\norm{\hat{e^{q\cdot}\partial_X^r[f]}}_{L^2}
+ \norm{\hat{e^{-q\cdot}\partial_X^r[f]}}_{L^2}\right) \\
\\
&= C_{r,q}\left(
\norm{e^{q\cdot}f}_{L^2}
+ \norm{e^{-q\cdot}f}_{L^2}
+ \norm{e^{q\cdot}\partial_X^r[f]}_{L^2}
+ \norm{e^{-q\cdot}\partial_X^r[f]}_{L^2}\right) \\
\\
&\le C_{r,q}\left(\norm{\cosh(q\cdot)f}_{L^2} + \norm{\cosh(q\cdot)\partial_X^r[f]}_{L^2}\right) \\
\\
&= C_{r,q}\triplenorm{f}_{r,q}.
\end{align*}
Hence
$$
\norm{f}_{\X_q^r} 
= \norm{\cosh(q\cdot)f}_{H^r} 
= \norm{\cosh(q\cdot)f}_{L^2} + \norm{\partial_X^r[\cosh(q\cdot)f]}_{L^2} 
\le C_{r,q}\triplenorm{f}_{r,q}.
$$

Now we show 
\begin{equation}\label{Hrq norm equiv induction}
\triplenorm{f}_{\X_q^r} \le C_{r,q}\norm{f}_{\X_q^r}
\end{equation}
by induction on $r$. We will use the essential inequality 
\begin{equation}\label{cosh ge sinh}
|\sinh(X)| 
= \left|\frac{e^X-e^{-X}}{2}\right|
\le \frac{e^X+e^{-X}}{2}
= \cosh(X)
\end{equation}
and the equality
$$
\partial_X[\cosh(\cdot)] = \sinh(\cdot).
$$
%and the formula
%\begin{equation}\label{leibniz coshq}
%\cosh(q\cdot)\partial_X^r[f] = \partial_X^r[\cosh(q\cdot)f] -\sum_{j=1}^r {r \choose j} \partial_X^j[\cosh(q\cdot)]\partial_X^{r-j}[f]
%\end{equation}
%from Leibniz' rule.

When $r=1$,
\begin{align*}
\norm{\cosh(q\cdot)\partial_X[f]}_{L^2} 
&\le \norm{\partial_X[\cosh(q\cdot)f]}_{L^2}
+ q\norm{\sinh(q\cdot)f}_{L^2} \\
\\
&\le \norm{\cosh(q\cdot)f}_{H^1} + q\norm{\cosh(q\cdot)f)}_{L^2} \\
\\
&\le (1+q)\norm{\cosh(q\cdot)f}_{H^1} \\
\\
&= (1+q)\norm{f}_{\X_q^1},
\end{align*}
and so
$$
\triplenorm{f}_{\X_q^1} \le (1+q)\norm{f}_{\X_q^1}.
$$ 

Assume that \eqref{Hrq norm equiv induction} holds for some $r \ge 1$. Then \eqref{leibniz consequence} gives
$$
\cosh(q\cdot)\partial_X^{r+1}[f]
= \partial_X^{r+1}[\cosh(q\cdot)f] - \sum_{j=1}^{r+1} {r+1 \choose j} \partial_X^j[\cosh(q\cdot)]\partial_X^{r+1-j}[f],
$$
where $\partial_X^{r+1}[\cosh(q\cdot)f] \in L^2$ and, for $1 \le j \le r+1$, we have $0 \le r+1-j \le r$, hence 
\begin{align*}
\norm{\partial_X^j[\cosh(q\cdot)]\partial_X^{r+1-j}[f]}_{L^2}
&\le q^j\norm{\cosh(q\cdot)\partial_X^{r+1-j}[f]}_{L^2} \\
\\
&\le q^j\triplenorm{f}_{\X_q^{r+1-j}} \\
\\
&\le C_{r,q,j}\norm{f}_{\X_q^{r+1-j}} \text{ by the induction hypothesis} \\
\\
&= C_{r,q,j}\norm{\cosh(q\cdot)f}_{H^{r+1-j}} \\
\\
&\le C_{r,q,j}\norm{\cosh(q\cdot)f}_{H^{r+1}} \text{by \eqref{sobolev lower higher bound}} \\
\\
&\le C_{r,q}\norm{f}_{\X_q^{r+1}}.  
\end{align*}
Thus
\begin{align*}
\norm{\cosh(q\cdot)\partial_X^{r+1}[f]}_{L^2}
&\le \norm{\partial_X^{r+1}[\cosh(q\cdot)f]}_{L^2} + C_{r,q}\norm{f}_{\X_q^{r+1}} \\
\\
&\le \norm{\cosh(q\cdot)f}_{H^{r+1}}+C_{r,q}\norm{f}_{\X_q^{r+1}} \\
\\
&\le C_{r,q}\norm{f}_{\X_q^{r+1}}.
\end{align*}
This shows both $\cosh(q\cdot)\partial_X^{r+1}[f] \in L^2$ and 
\begin{equation}\label{Xqr+1 equiv forward}
\triplenorm{f}_{\X_q^{r+1}}
= \norm{\cosh(q\cdot)f}_{L^2} + \norm{\cosh(q\cdot)\partial_X^{r+1}[f]}_{L^2}
\le C_{r,q}\norm{f}_{\X_q^{r+1}}.
\end{equation}
\end{proof}

\begin{lemma}\label{Yrq equivalence lemma}
The norms $\norm{\cdot}_{\Y_q^r}$ and $\triplenorm{\cdot}_{\Y_q^r}$ are equivalent on $H_q^r$.
\end{lemma}

\begin{proof}
The proof both relies on and has much in common with the proof of \ref{Xrq norm equivalence}, except now the key inequality is not \eqref{cosh ge sinh} but 
$$
|\partial_X^r[\cosh^q(\cdot)]| \le C_{r,q}\cosh^q(\cdot),
$$
per Lemma \ref{cosh power q ineq} below. Then
\begin{align*}
\norm{\partial_X^r[\cosh^q(\cdot)f]}_{L^2}
&\le C_r\sum_{j=0}^r \norm{\partial_X^j[\cosh^q(\cdot)]\partial_X^{r-j}[f]}_{L^2} \\
\\
&\le C_{r,q}\sum_{j=0}^r \norm{\cosh^q(\cdot)\partial_X^j[f]}_{L^2} \\
\\
&\le C_{r,q}\sum_{j=0}^r \norm{\cosh(q\cdot)\partial_X^j[f]}_{L^2} \\
\\
&\le C_{r,q}\sum_{j=0}^r \triplenorm{f}_{\X_q^j} \\
\\
&\le C_{r,q}\sum_{j=0}^r \norm{f}_{\X_q^j} \\
\\
&\le C_{r,q}\norm{f}_{\X_q^r} \text{ by \eqref{sobolev lower higher bound}} \\
\\
&\le C_{r,q}\triplenorm{f}_{\X_q^r} \\
\\
&\le C_{r,q}\triplenorm{f}_{\Y_q^r}.
\end{align*}
Hence there is $C_{r,q} > 0$ such that 
$$
\norm{f}_{\Y_q^r} \le C_{r,q}\triplenorm{f}_{\Y_q^r}, \ f \in H_q^r.
$$

For the other inequality, we induct.  When $r=1$, we have
\begin{align*}
\norm{\cosh^q(\cdot)f'}_{L^2}
&\le \norm{\partial_X[\cosh^q(\cdot)f]}_{L^2} + \norm{\partial_X[\cosh^q(\cdot)]f}_{L^2} \\
\\
&\le \norm{\partial_X[\cosh^q(\cdot)f]}_{L^2} + C_q\norm{\cosh^q(\cdot)f}_{L^2} \\
\\
&\le C_q\norm{f}_{\Y_q^1}.
\end{align*}
Assume there are $r \ge 1$ and $C_{j,q} > 0$ such that 
$$
\triplenorm{f}_{\Y_q^j} \le C_{j,q}\norm{f}_{\Y_q^j}, \ j = 0,\ldots,r.
$$
Then
\begin{align*}
\norm{\cosh^q(\cdot)\partial_X^{r+1}[f]}_{L^2}
&\le C_r\sum_{j=0}^r \norm{\partial_X[\cosh^q(\cdot)]\partial_X^{r+1-j}[f]}_{L^2} \\
\\
&\le C_{r,q}\sum_{j=0}^r \norm{\cosh^q(\cdot)\partial_X^j[f]}_{L^2} \\
\\
&\le C_{r,q}\sum_{j=0}^r \triplenorm{f}_{\Y_q^j} \\
\\
&\le C_{r,q}\sum_{j=0}^r \norm{f}_{\Y_q^j} \\
\\
&\le C_{r,q}\norm{f}_{\Y_q^{r+1}} \text{ by \eqref{sobolev lower higher bound}}.
\end{align*}
\end{proof}
%
%%%%------------------------------------------------------------------------------------------------------------------------------------------------------------------------------------------------------------%%
%%%%------------------------------------------------------------------------------------------------------------------------------------------------------------------------------------------------------------%%
%%\begin{proposition}
%%\end{proposition}
%%
%%\begin{proof}
%%This is largely the same as the proof of Proposition \ref{Xrq equiv}.
%%\end{proof}

%%------------------------------------------------------------------------------------------------------------------------------------------------------------------------------------------------------------%%
%%------------------------------------------------------------------------------------------------------------------------------------------------------------------------------------------------------------%%
\begin{lemma}\label{cosh equiv lemma}
For all $q > 0$ there exists a constant $C_q > 0$ such that 
\begin{equation}\label{cosh equiv}
\frac{1}{C_q}\cosh(qX) \le \cosh^q(X) \le C_q\cosh(qX), \ X \in \R.
\end{equation}
\end{lemma}

\begin{proof} %(Formal)
Recall that if $A,B > 0$, then
\begin{equation}\label{basic q power ineq}
(A+B)^q \le 2^q(A^q+B^q).
\end{equation}
Then
$$
\cosh^q(X) = \frac{1}{2^q}(e^X+e^{-X})^q \le e^{qX}+e^{-qX} = 2\cosh(qX).
$$

For the first inequality in \eqref{cosh equiv}, set
$$
f(X) = \cosh^q(X)-\frac{1}{c}\cosh(qX),
$$
where
$$
c = q2^{q-1}+2.
$$
Then 
$$
f(0) = 1-\frac{1}{c} > 0 
$$
since $c > 1$. We will show that $f'(X) > 0$ for $X > 0$, which means that $f$ is increasing on $(0,\infty)$, and therefore $f(X) \ge 0$ for $X > 0$.  And since $f$ is even, this means $f(X) \ge 0$ for all $X$.  Then we will have the first inequality in \eqref{cosh equiv}.

We compute
$$
f'(X) = q\cosh^{q-1}(X)\sinh(X)-\frac{q}{c}\sinh(qX),
$$
so $f'(X) > 0$ if and only if
$$
0 < \left(\frac{e^X+e^{-X}}{2}\right)^{q-1}(e^X-e^{-X})-\frac{1}{c}(e^{qX}-e^{-qX})
$$
Since $e^X-e^{-X} > 0$ for $X > 0$, this rearranges to
\begin{equation}\label{goal}
f'(X) > 0 \iff \frac{2^{q-1}}{c}\frac{e^{qX}-e^{-qX}}{e^X-e^{-X}} < (e^X+e^{-X})^{q-1}.
\end{equation}
Set 
$$
g(Y) = Y^q.
$$
The mean value theorem implies
\begin{align*}
\frac{e^{qX}-e^{-qX}}{e^X-e^{-X}} 
&= \frac{g(e^X)-g(e^{-X})}{e^X-e^{-X}} \\
\\
&\le \max_{e^{-X} \le Y \le e^X} g'(Y) \\
\\
&= q\max_{e^{-X}\le Y \le e^X} Y^{q-1} \\
\\
&= \begin{cases}
qe^{(1-q)X}, &0 < q < 1 \\
qe^{(q-1)X}, &q \ge 1.
\end{cases}
\end{align*}
When $0 < q < 1$, we have
$$
e^{(1-q)X} 
= (e^X)^{1-q}
< (e^X+e^{-X})^{1-q}
$$
and likewise
$$
e^{(q-1)X} < (e^X+e^{-X})^{q-1}
$$
when $q \ge 1$. So, for any $q > 1$, we find
$$
\frac{e^{qX}-e^{-qX}}{e^X-e^{-X}} \le q(e^X+e^{-X})^{q-1}.
$$
Then
\begin{align*}
\frac{2^{q-1}}{c}\frac{e^{qX}-e^{-qX}}{e^X-e^{-X}} 
&\le \frac{2^{q-1}q}{c}(e^X+e^{-X})^{q-1} \\
\\
&= \frac{q2^{q-1}}{q2^{q-1}+2}(e^X+e^{-X})^{q-1} \\
\\
&< (e^X+e^{-X})^{q-1},
\end{align*}
and this is \eqref{goal}, which implies $f'(X) > 0$ for any $X > 0$.
\end{proof}

An immediate consequence of this lemma is that, for any $g \in L^2$, we have $\cosh(q\cdot)g \in L^2$ if and only if $\cosh^q(\cdot)g \in L^2$.  In particular, given $f \in H^r$, we have $\cosh(q\cdot)\partial_X^k[f] \in L^2$ if and only if $\cosh^q(\cdot)\partial_X^k[f] \in L^2$, $k=0,r$.  Hence $\X_q^r = \Y_q^r$ and $\triplenorm{\cdot}_{\X_q^r}$ and $\triplenorm{\cdot}_{\Y_q^r}$ are equivalent. The equivalence of the norms $\norm{\cdot}_{\X_q^r}$ and $\triplenorm{\cdot}_{\X_q^r}$ from Lemma \ref{Xrq norm equivalence} and the norms $\norm{\cdot}_{\Y_q^r}$ and $\triplenorm{\cdot}_{\Y_q^r}$ from Lemma \ref{Yrq equivalence lemma} then complete the proof of Theorem \ref{weighted equiv theorem}.

% Moreover, by Lemma \ref{cosh equiv}
%\begin{multline*}
%\norm{f}_{\X_q^r} 
%\le C_{r,q}\triplenorm{f}_{\X_q^r} 
%= C_{r,q}\sum_{k=0}^r \norm{\cosh(q\cdot)\partial_X^k[f]}_{L^2} 
%\le C_{r,q}\sum_{k=0}^r \norm{\cosh^q(\cdot)\partial_X^k[f]}_{L^2} \\
%= \triplenorm{f}_{\Y_q^r} 
%\le C_{r,q}\norm{f}_{\Y_q^r}.
%\end{multline*}
%The proof of the inequality $\norm{f}_{\Y_q^r} \le C_{q,r}\norm{f}_{\X_q^r}$ is identical, and this completes the proof that $\X_q^r = \Y_q^r$ and $\norm{\cdot}_{\X_q^r}$ and $\norm{\cdot}_{\Y_q^r}$ are equivalent.  

%%------------------------------------------------------------------------------------------------------------------------------------------------------------------------------------------------------------%%
%%------------------------------------------------------------------------------------------------------------------------------------------------------------------------------------------------------------%%
%%------------------------------------------------------------------------------------------------------------------------------------------------------------------------------------------------------------%%
\subsubsection{Lemmas for the proof of the equivalent norms} 

%%------------------------------------------------------------------------------------------------------------------------------------------------------------------------------------------------------------%%
%%------------------------------------------------------------------------------------------------------------------------------------------------------------------------------------------------------------%%
\begin{lemma}
Let $r > 0$.  Then 
\begin{equation}\label{j r domination}
|k|^j < 1+|k|^r
\end{equation}
for all $k \in \mathbb{C}$ and $j \in [0,r]$.
\end{lemma}

\begin{proof}
If $|k| < 1$, then
$$
|k|^j < 1 < 1+|k|^r,
$$
and if $|k| \ge 1$, then
\[
|k|^j \le |k|^r < 1 + |k|^r.
\qedhere
\]
\end{proof}

%%------------------------------------------------------------------------------------------------------------------------------------------------------------------------------------------------------------%%
%%------------------------------------------------------------------------------------------------------------------------------------------------------------------------------------------------------------%%
\begin{lemma}\label{lemma for q ft deriv}
Let $\cosh(q\cdot)f \in H^r$.  Then
\begin{enumerate}[label={\bf(\roman*)}]
%%------------------------------------------------------------------------------------------------------------------------------------------------------------------------------------------------------------%%
\item $\cosh(q\cdot)\partial_X^j[f] \in L^2$, $j = 0,\ldots,r$
%%------------------------------------------------------------------------------------------------------------------------------------------------------------------------------------------------------------%%
\item $\lim_{y \to q} \norm{(e^{y\cdot}-e^{q\cdot})f}_{H^r} = 0$.
\end{enumerate}
\end{lemma}

\begin{proof}
\begin{enumerate}[label={\bf(\roman*)}]
%%------------------------------------------------------------------------------------------------------------------------------------------------------------------------------------------------------------%%
\item We will use the following identity from Leibniz' rule frequently:
\begin{equation}\label{leibniz consequence}
\cosh(q\cdot)\partial_X^j[f] = \partial_X^j[\cosh(q\cdot)f] - \sum_{\ell=1}^j {j \choose \ell} \partial_X^{\ell}[\cosh(q\cdot)]\partial_X^{j-\ell}[f].
\end{equation}
We induct on $r$. $f \in H_q^1$, then
$$
\cosh(q\cdot)f' = \partial_X[\cosh(q\cdot)f] - q\sinh(q\cdot)f,
$$
hence 
$$
\norm{\cosh(q\cdot)f'}_{L^2}
\le \norm{\partial_X[\cosh(q\cdot)f]}_{L^2} + q\norm{\sinh(q\cdot)f}_{L^2}
\le \norm{f}_{1,q}+q\norm{\cosh(q\cdot)f}_{L^2}
\le (1+q)\norm{f}_{1,q}.
$$
Assume the result is true for some $r \ge 1$.  Then $f \in H_q^{r+1}$ implies $f \in H_q^r$, so $\cosh(q\cdot)\partial_X^j[f] \in L^2$ for $j=0,\ldots,r$.  We check the $j=r+1$ case: 
$$
\cosh(q\cdot)\partial_X^{r+1}[f] 
= \partial_X^{r+1}[\cosh(q\cdot)f] - \sum_{\ell=1}^{r+1} {r+1 \choose \ell} \partial_X^{\ell}[\cosh(q\cdot)]\partial_X^{r+1-\ell}[f].
$$
We have $\partial_X^{r+1}[\cosh(q\cdot)f] \in L^2$ by hypothesis and 
$$
\norm{\partial_X^{\ell}[\cosh(q\cdot)]\partial_X^{r+1-\ell}}_{L^2}
\le q^{\ell}\norm{\cosh(q\cdot)\partial_X^{r+1-\ell}}_{L^2}
$$
by \eqref{leibniz consequence}, where $1 \le \ell \le r+1$ means $0 \le r+1-\ell \le r$.  Hence $\cosh(q\cdot)\partial_X^{r+1-\ell}[f] \in L^2$.  

%%------------------------------------------------------------------------------------------------------------------------------------------------------------------------------------------------------------%%
\item We need to take limits on two $L^2$-norms:
$$
\norm{(e^{y\cdot}-e^{q\cdot})f}_{H^r}
= \norm{(e^{y\cdot}-e^{q\cdot})f}_{L^2}
+ \norm{\partial_X^r[(e^{y\cdot}-e^{q\cdot})f]}_{L^2}.
$$
The pointwise convergence to 0 as $y \to q$ is obvious, so we check for domination: first,
$$
\norm{(e^{y\cdot}-e^{q\cdot})f}_{L^2}
\le \norm{e^{y\cdot}f}_{L^2} + \norm{e^{q\cdot}f}_{L^2}
\le 2\norm{c_yf}_{L^2}+2\norm{\cosh(q\cdot)f}_{L^2}
\le 4\norm{\cosh(q\cdot)f}_{L^2},
$$
where we are using the inequality
$$
e^{yx} 
= 2\frac{e^{yx}}{2}
\le 2\frac{e^{yx}+e^{-yx}}{2}
= 2\cosh(yx)
\le 2\cosh(qx).
$$
Also, and similarly,
\begin{align*}
\norm{\partial_X^r[(e^{y\cdot}-e^{q\cdot})f]}_{L^2}
&\le \sum_{j=0}^r {r \choose j}\norm{(y^je^{y\cdot}-q^je^{q\cdot})\partial_X^{r-j}[f]}_{L^2} \\
\\
&\le C_r\sum_{j=0}^r \left(|y|^j\norm{e^{y\cdot}\partial_X^{r-j}[f]}_{L^2}+q^j\norm{e^{q\cdot}\partial_X^{r-j}[f]}_{L^2}\right) \\
\\
&\le C_r\sum_{j=0}^r q^j\norm{\cosh(q\cdot)\partial_X^{r-j}[f]}_{L^2}.
\end{align*}
So, the limit follows from the dominated convergence theorem.
\qedhere
\end{enumerate}
\end{proof}

With these lemmas, we can show that we preserve the familiar identity for the derivative when we extend the Fourier transform to complex values: if $\cosh(q\cdot)f \in H^r$ for some integer $r \ge 1$, then 
$$
\ft[\partial_X^rf](z) = (iz)^r\hat{f}(z), \ z \in \overline{\Sigma}_q,.
$$
where $\overline{\Sigma}_q$ is the closure of $\Sigma_q$ (as in Theorem \ref{eigenprops}).  The proof for $|\im(z)| < q$ is Theorem 8.4.4 in \cite{dettman}.  We prove the $|\im(z)| = q$ case here as an equality in $L^2$.

%%------------------------------------------------------------------------------------------------------------------------------------------------------------------------------------------------------------%%
%%------------------------------------------------------------------------------------------------------------------------------------------------------------------------------------------------------------%%
\begin{proposition}
Let $f \in H_q^r$.  Then $\hat{\partial_X^j[f]}(k\pm iq) = (i(k\pm iq))^j\hat{f}(k\pm iq)$.
\end{proposition}

\begin{proof}
Since $H_q^r \subseteq H_q^{r-1}$, we give the proof just for $j=r$.  Let $|y| < q$.  |We have
$$\
\hat{\partial_X^jf}(k+iq) - (i(k+iq))^j\hat{f}(k+iq)
=
\bunderbrace{\hat{\partial_X^jf}(k+iq)-\hat{\partial_X^jf}(k+iy)}{\Delta_1(k,y)}
+\bunderbrace{\hat{\partial_X^jf}(k+iy)-(i(k+iq))^j\hat{f}(k+iq)}{\Delta_2(k,y)}.
$$
Immediately \eqref{lim y to q ft complex} gives
$$
\lim_{y \to q} \norm{\Delta_1(\cdot,y)}_{L^2} = 0.
$$

Next, rewrite $\Delta_2(y)$ as
$$
\Delta_2(y)
= \bunderbrace{(i(k+iy))^j\hat{f}(k+iy)-(i(k+iy))^j\hat{f}(k+iq)}{\Delta_3(k,y)} 
+ \bunderbrace{(i(k+iy))^j\hat{f}(k+iq)-(i(k+iq))^j\hat{f}(k+iq)}{\Delta_4(k,y)}.
$$
Then \eqref{j r domination} implies
\begin{align*}
|\Delta_3(k,y)|
&= i^j\sum_{\ell=0}^j {j \choose \ell} k^{\ell}(-y)^{j-\ell}\left(\hat{e^{y\cdot}f}(k)-\hat{e^{q\cdot}f}(k)\right) \\
\\
&\le C_{r,q}\left(\left|\hat{e^{y\cdot}f}(k)-\hat{e^{q\cdot}f}(k)\right| + \left|(ik)^r\left(\hat{e^{y\cdot}f}(k)-\hat{e^{q\cdot}f}(k)\right)\right|\right) \\
\\
&= C_{r,q}\left(\left|\hat{(e^{y\cdot}-e^{q\cdot})f}(k)\right| + \left|\hat{\partial_X^r[(e^{y\cdot}-e^{q\cdot})f]}(k)\right|\right),
\end{align*}
and so
\begin{align*}
\norm{\Delta_3(\cdot,y)}_{L^2}
&\le C_{r,q}\left(\norm{\hat{(e^{y\cdot}-e^{q\cdot})f}}_{L^2}+\norm{\hat{\partial_X^r[(e^{y\cdot}-e^{q\cdot})f]}}_{L^2}\right) \\
\\
&= C_{r,q}\left(\norm{(e^{y\cdot}-e^{q\cdot})f}_{L^2} + \norm{\partial_X^r[(e^{y\cdot}-e^{q\cdot})]}_{L^2}\right) \\
\\
&= C_{r,q}\norm{(e^{y\cdot}-e^{q\cdot})f}_{H^r}.
\end{align*}
Hence $\norm{\Delta_3(\cdot,y)}_{L^2} \to 0$ as $y \to q$ by Lemma \ref{lemma for q ft deriv}.

Last, we rewrite 
\begin{align*}
\Delta_4(k,y)
&= i^j\left((k+iy)^j-(k+iq)^j\right)\hat{f}(k+iq) \\
\\
&= i^j\sum_{\ell=0}^j \left(k^{\ell}(iy)^{j-\ell}-k^{\ell}(iq)^{j-\ell}\right)\hat{e^{q\cdot}f}(k) 
\end{align*}
and so
\begin{align*}
\norm{\Delta_4(\cdot,y)}_{L^2}
&\le C_r\sum_{\ell=0}^j |y^{j-\ell}-q^{j-\ell}|\int_{\R} (1+k^2)^r\left|\hat{e^{q\cdot}f}(k)\right|^2 \dk \\
\\
&= C_r\sum_{\ell=0}^j |y^{j-\ell}-q^{j-\ell}|\norm{e^{q\cdot}f}_{H^r}
\end{align*}
Then $\norm{\Delta_4(\cdot,y)}_{L^2} \to 0$ as $y \to q$.
\end{proof}

%%------------------------------------------------------------------------------------------------------------------------------------------------------------------------------------------------------------%%
%%------------------------------------------------------------------------------------------------------------------------------------------------------------------------------------------------------------%%
\begin{lemma}\label{cosh power q ineq}
For all $r,q \ge 0$, there is a constant $C_{r,q} > 0$ such that
\begin{equation}\label{coshq ineq}
|\partial_X^r[\cosh^q(\cdot)]| \le C_{r,q}\cosh^q(\cdot).
\end{equation}
\end{lemma}

\begin{proof}
Use Fa\'{a} di Bruno's rule with $N(X) = X^q$ to write
\begin{equation}\label{coshq FdB}
\partial_X^r[\cosh^q(\cdot)] 
= \sum_{k=1}^r \left(\prod_{j=0}^{k-1} q-k\right)\cosh^{q-k}(\cdot)\sum_{\sigmab \in \Sigma_k^r}\prod_{j=1}^k \partial_X^{\sigma_j}[\cosh(\cdot)]
%= \sum_{\sigmab \in \Sigma_r} C_{\sigmab}\left(\prod_{j=0}^{|\sigmab|} q-j\right)\cosh^{q-|\sigmab|}(\cdot)\prod_{\ell=1}^k \left(\partial_X^{\ell}[\cosh(\cdot)]\right)^{\sigma_{\ell}},
\end{equation}
and observe that since $\cosh(X) \ge 0$,
$$
\left|\prod_{\ell=1}^k  \partial_X^{\sigma_j}[\cosh(\cdot)]\right| 
\le \prod_{\ell=1}^k \cosh(\cdot)
=\cosh^k(\cdot).
$$
This and \eqref{coshq FdB} imply the desired inequality \eqref{coshq ineq}.
\end{proof}
