# Supplementary material for: Nanopteron-stegoton traveling waves in spring dimer Fermi-Pasta-Ulam-Tsingou lattices
Source: arXiv:1710.07376 source file (2017-10-20)
Supplement: Supplementary file 4 [file appendix_sobolev_spaces_estimates.tex]

%%------------------------------------------------------------------------------------------------------------------------------------------------------------------------------------------------------------%%
%%------------------------------------------------------------------------------------------------------------------------------------------------------------------------------------------------------------%%
%%------------------------------------------------------------------------------------------------------------------------------------------------------------------------------------------------------------%%
\subsubsection{Estimates for $H_q^r$} 
